# Supplementary material for: Triangle Preferential Attachment Has Power-law Degrees and Eigenvalues; Eigenvalues Are More Stable to Network Sampling
Source: arXiv:1904.12989 source file (2019-04-29)
Supplement: Supplementary file 1 [file 90-Appendix.tex]

\section{Supplement}
\label{sec:appendix}
%To conclude this manuscript, we provide proofs for theoretical results from Section~\ref{sec:GPAResults}.
\input{proof-lemma1}
\input{proof-lemma2}
\input{proof-theorem1}
